# Supplementary material for: Seismic wavefield solutions via physics-guided generative neural operator
Source: arXiv:2503.06488 source file (2025-03-09)
Supplement: Supplementary file 1 [file Appendix.tex]

\section{\textsc{SUPPLEMENTARY INFORMATION}}
% \vspace{8pt} \\ 
Supporting information for section X
